# Supplementary material for: Best of Both Worlds Guarantees for Equitable Allocations
Source: arXiv:2505.05809 source file (2025-05-09)
Supplement: Supplementary file 1 [file appendix.tex]

\newpage

\appendix
